# Supplementary material for: Topological EEG Nonlinear Dynamics Analysis for Emotion Recognition
Source: arXiv:2203.06895 source file (2022-03-14)
Supplement: Supplementary file 1 [file Appendix.pdf]

# Topological EEG Nonlinear Dynamics Analysis for Emotion Recognition (Appendix)

In this work, we evaluate the model with two public datasets, namely the DEAP and the DREAMER dataset. According to the settings described in the experiments section, we provide the detailed results for each subject for further investigation and referee. In Table A.I, A.II, and A.III we present the results of Exp. #1 and #2 as noted in the body manuscript of this work, which include the  $\theta$ ,  $\alpha$ ,  $\beta$ , and  $\gamma$  band-based results performed on DEAP and DREAMER (based on 1s window size and 25% overlap). In Table A.IV, A.V, A.VI, and A.VII we illustrate the results of the TEEGND model performed on DEAP with sliding windows equal to 0.5s, 2s, 3s, and 4s (Exp. #3). Meanwhile, Table A.VIII, A.IX, A.X, and A.XI include the experiment results of DREAMER dataset performed with 0.5s, 2s, 3s, and 4s sliding window sizes of EEG. It is worth mentioning that in the 3s-window based experiments we use the overlap percentage as 0% for comparison purposed with other related work, and 0.5s-window based with non-overlapping for short-term recognition. This ad-hoc setting would not affect our main conclusion of our proposed approach.

TABLE A.I  
EXPERIMENTS WITH TEEGND A WITH RHYTHM BAND COMPARISONS PERFORMED ON DEAP (1s-WINDOW, 25% OVERLAP).

| ID | No. of Valence | $\theta$ -V(%) | $\alpha$ -V(%) | $\beta$ -V(%) | $\gamma$ -V(%) | All-V (%) | No. of Arousal | $\theta$ -A(%) | $\alpha$ -A(%) | $\beta$ -A(%) | $\gamma$ -A(%) | All-A(%) |
|----|----------------|----------------|----------------|---------------|----------------|-----------|----------------|----------------|----------------|---------------|----------------|----------|
| 01 | 1743:1577      | 99.73          | 99.79          | 79.91         | 89.67          | 99.97     | 1328:1992      | 99.88          | 99.64          | 79.49         | 89.34          | 99.91    |
| 02 | 1494:1826      | 95.30          | 99.07          | 79.67         | 78.67          | 98.49     | 1328:1992      | 95.72          | 98.55          | 76.48         | 78.80          | 99.13    |
| 03 | 1494:1826      | 97.23          | 99.34          | 72.29         | 81.36          | 98.73     | 2656:664       | 95.75          | 99.28          | 82.56         | 83.83          | 98.95    |
| 04 | 1992:1328      | 90.48          | 96.84          | 80.24         | 79.07          | 95.66     | 1922:1328      | 90.45          | 96.78          | 77.89         | 81.60          | 97.05    |
| 05 | 1328:1992      | 96.48          | 98.70          | 88.92         | 92.89          | 99.40     | 1743:1577      | 96.11          | 98.92          | 88.80         | 88.61          | 99.34    |
| 06 | 830:2490       | 98.95          | 99.61          | 79.52         | 82.05          | 99.70     | 1909:1411      | 99.28          | 99.85          | 76.57         | 77.50          | 99.94    |
| 07 | 996:2324       | 99.58          | 99.85          | 77.47         | 79.31          | 99.94     | 1245:2075      | 99.76          | 100            | 80.66         | 76.17          | 100      |
| 08 | 1494:1826      | 97.56          | 99.70          | 89.94         | 91.01          | 99.94     | 1411:1909      | 97.71          | 99.37          | 88.52         | 92.56          | 99.79    |
| 9  | 1660:1660      | 97.17          | 99.31          | 80.63         | 83.43          | 99.46     | 1328:1992      | 97.05          | 99.31          | 79.67         | 83.95          | 99.40    |
| 10 | 1660:1660      | 98.73          | 99.43          | 85.81         | 92.29          | 99.16     | 1494:1826      | 98.07          | 99.16          | 79.94         | 89.46          | 99.82    |
| 11 | 1328:1992      | 95.39          | 96.36          | 73.25         | 81.02          | 97.80     | 2075:1245      | 96.57          | 96.93          | 70.39         | 82.98          | 97.77    |
| 12 | 1577:1743      | 99.13          | 99.94          | 77.20         | 84.01          | 99.76     | 581:2739       | 98.46          | 99.67          | 88.10         | 88.86          | 99.73    |
| 13 | 1909:1411      | 99.16          | 99.15          | 81.42         | 86.17          | 99.64     | 498:2822       | 98.7           | 99.31          | 89.67         | 91.51          | 99.40    |
| 14 | 1600:1600      | 98.70          | 99.79          | 78.55         | 79.28          | 99.67     | 1079:2241      | 97.89          | 99.25          | 80.18         | 77.41          | 99.31    |
| 15 | 1600:1600      | 99.01          | 99.91          | 90.78         | 93.58          | 99.85     | 1743:1577      | 99.13          | 99.82          | 90.33         | 91.93          | 99.94    |
| 16 | 1245:2075      | 97.83          | 99.61          | 83.67         | 83.61          | 99.94     | 1600:1600      | 99.49          | 99.82          | 84.55         | 86.20          | 99.94    |
| 17 | 1826:1494      | 98.49          | 99.37          | 87.02         | 91.20          | 99.64     | 1328:1992      | 97.89          | 98.64          | 86.69         | 92.47          | 99.31    |
| 18 | 1328:1992      | 99.64          | 99.40          | 83.19         | 89.97          | 99.85     | 1245:2075      | 99.52          | 99.46          | 84.37         | 86.27          | 99.79    |
| 19 | 1411:1909      | 96.36          | 99.61          | 83.49         | 86.39          | 99.82     | 1079:2241      | 96.30          | 99.07          | 85.93         | 86.51          | 99.37    |
| 20 | 1411:1909      | 99.43          | 99.52          | 82.26         | 88.55          | 99.76     | 747:2573       | 99.28          | 99.46          | 84.64         | 91.69          | 99.67    |
| 21 | 1577:1743      | 99.67          | 99.76          | 80.78         | 76.72          | 99.73     | 664:2656       | 97.95          | 99.37          | 85.75         | 83.46          | 99.28    |
| 22 | 1826:1494      | 87.53          | 96.66          | 97.32         | 88.34          | 97.68     | 1328:1992      | 86.81          | 96.90          | 87.53         | 87.98          | 98.86    |
| 23 | 1162:2158      | 99.91          | 99.97          | 90.00         | 88.83          | 99.97     | 2490:830       | 99.91          | 99.94          | 92.41         | 93.16          | 99.82    |
| 24 | 1826:1494      | 92.47          | 99.25          | 69.31         | 81.14          | 98.92     | 581:2739       | 95.06          | 99.07          | 83.35         | 87.92          | 98.80    |
| 25 | 1743:1577      | 94.28          | 97.89          | 77.32         | 80.54          | 98.55     | 913:2407       | 95.24          | 97.83          | 79.34         | 82.65          | 97.44    |
| 26 | 1162:2158      | 96.99          | 99.19          | 90.81         | 93.58          | 99.85     | 1909:1411      | 95.15          | 99.40          | 97.14         | 91.08          | 99.85    |
| 27 | 830:2490       | 99.73          | 99.88          | 90.42         | 92.71          | 99.91     | 1079:2241      | 99.79          | 99.70          | 87.05         | 90.24          | 99.79    |
| 28 | 1245:2075      | 97.56          | 99.22          | 73.67         | 82.14          | 99.13     | 1826:1494      | 98.61          | 99.40          | 72.05         | 81.14          | 99.64    |
| 29 | 1411:1909      | 98.89          | 99.61          | 90.87         | 92.80          | 99.91     | 1245:2075      | 98.49          | 99.43          | 91.14         | 93.64          | 99.85    |
| 30 | 1037:2241      | 97.92          | 98.77          | 82.23         | 87.50          | 99.49     | 1743:1577      | 98.22          | 99.61          | 81.84         | 87.71          | 99.67    |
| 31 | 1411:1909      | 99.46          | 99.76          | 78.40         | 90.30          | 99.97     | 1743:1577      | 99.34          | 99.85          | 79.40         | 89.73          | 99.97    |
| 32 | 1660:1660      | 96.93          | 99.76          | 80.21         | 74.91          | 99.85     | 1079:2241      | 95.90          | 99.49          | 82.95         | 77.77          | 99.19    |

TABLE A.II  
EXPERIMENTS WITH TEEGENDA WITH RHYTHM BAND COMPARISONS PERFORMED ON DREAMER (VALENCE AND AROUSAL, 1s-WINDOW, 25% OVERLAP) - I.

| ID | No. of Valence | $\theta$ -V(%) | $\alpha$ -V(%) | $\beta$ -V(%) | $\gamma$ -V(%) | All-V(%) | No. of Arousal | $\theta$ -A(%) | $\alpha$ -A(%) | $\beta$ -A(%) | $\gamma$ -A(%) | All-A(%) |
|----|----------------|----------------|----------------|---------------|----------------|----------|----------------|----------------|----------------|---------------|----------------|----------|
| 01 | 2628:2332      | 98.27          | 96.79          | 99.09         | 98.85          | 99.84    | 3404:1556      | 98.37          | 97.18          | 98.53         | 98.04          | 99.80    |
| 02 | 3384:1576      | 99.98          | 100            | 99.42         | 99.19          | 99.90    | 2082:2878      | 100            | 99.98          | 98.85         | 98.65          | 99.98    |
| 03 | 2541:2419      | 99.98          | 99.94          | 97.96         | 95.81          | 100      | 2641:2319      | 99.94          | 99.94          | 96.90         | 96.43          | 100      |
| 04 | 3808:1152      | 99.66          | 99.19          | 99.58         | 99.48          | 99.70    | 3409:1551      | 99.48          | 97.38          | 99.66         | 99.42          | 99.74    |
| 05 | 3119:1841      | 99.86          | 99.64          | 95.91         | 96.79          | 99.96    | 2240:2720      | 99.72          | 99.78          | 95.77         | 95.89          | 99.94    |
| 06 | 2697:2263      | 100            | 99.98          | 99.23         | 98.67          | 99.96    | 1524:3436      | 100            | 100            | 99.09         | 98.53          | 99.98    |
| 07 | 3252:1708      | 99.92          | 100            | 99.05         | 98.63          | 99.88    | 2991:1969      | 99.94          | 99.92          | 98.45         | 97.88          | 100      |
| 08 | 3279:1681      | 99.90          | 100            | 99.40         | 99.42          | 99.98    | 3575:1385      | 99.88          | 100            | 99.52         | 98.99          | 99.90    |
| 09 | 2770:2190      | 99.98          | 99.94          | 98.67         | 98.02          | 99.98    | 1384:3576      | 99.94          | 99.98          | 99.60         | 99.09          | 100      |
| 10 | 1869:3091      | 100            | 99.40          | 99.70         | 99.23          | 99.92    | 3054:1906      | 99.80          | 99.82          | 99.48         | 99.19          | 99.96    |
| 11 | 3203:1757      | 100            | 99.98          | 99.66         | 99.09          | 99.98    | 2817:2143      | 99.60          | 99.94          | 99.56         | 98.83          | 100      |
| 12 | 2426:2534      | 100            | 99.80          | 96.92         | 96.90          | 99.96    | 2524:2436      | 100            | 100            | 96.33         | 95.56          | 99.98    |
| 13 | 2164:2796      | 99.96          | 99.70          | 98.73         | 98.29          | 100      | 2491:2469      | 99.82          | 99.23          | 97.30         | 95.91          | 100      |
| 14 | 2758:2202      | 100            | 100            | 94.11         | 94.25          | 99.98    | 3036:1924      | 100            | 100            | 97.34         | 92.70          | 100      |
| 15 | 3252:1708      | 100            | 99.88          | 98.89         | 98.79          | 99.88    | 2312:2648      | 99.84          | 99.98          | 99.25         | 98.71          | 99.98    |
| 16 | 3125:1835      | 99.88          | 99.86          | 99.09         | 98.31          | 99.84    | 2247:2713      | 99.70          | 99.90          | 97.82         | 98.53          | 99.88    |
| 17 | 3210:1750      | 99.94          | 99.88          | 97.32         | 96.07          | 99.90    | 3521:1439      | 99.96          | 99.86          | 98.49         | 97.56          | 99.94    |
| 18 | 3125:1835      | 100            | 99.98          | 95.67         | 92.20          | 100      | 2149:2811      | 100            | 100            | 95.32         | 90.97          | 100      |
| 19 | 2360:2600      | 99.92          | 99.96          | 98.95         | 96.90          | 99.90    | 800:4160       | 99.98          | 99.98          | 99.07         | 96.29          | 99.98    |
| 20 | 3323:1637      | 99.78          | 99.78          | 97.64         | 97.34          | 100      | 3079:1881      | 99.86          | 99.62          | 99.40         | 99.56          | 100      |
| 21 | 3107:1853      | 99.94          | 99.94          | 97.96         | 97.80          | 99.96    | 1547:3413      | 99.96          | 99.90          | 98.67         | 99.05          | 99.96    |
| 22 | 3134:1826      | 99.94          | 99.94          | 97.26         | 97.16          | 99.98    | 3130:1830      | 99.96          | 100            | 94.78         | 96.69          | 99.96    |
| 23 | 2685:2275      | 99.98          | 100            | 98.85         | 97.74          | 100      | 3444:1516      | 99.98          | 99.98          | 98.47         | 98.08          | 100      |

TABLE A.III  
EXPERIMENTS WITH TEEGENDA WITH RHYTHM BAND COMPARISONS PERFORMED ON DREAMER (DOMINANCE, 1s-WINDOW, 25% OVERLAP) - II.

| ID | No. of Dominance | $\theta$ -D(%) | $\alpha$ -D(%) | $\beta$ -D(%) | $\gamma$ -D(%) | All-D(%) |
|----|------------------|----------------|----------------|---------------|----------------|----------|
| 01 | 1955:3005        | 99.92          | 99.70          | 98.87         | 98.12          | 99.92    |
| 02 | 1915:3045        | 100            | 100            | 98.85         | 97.86          | 99.94    |
| 03 | 2920:2040        | 99.96          | 100            | 96.25         | 96.81          | 100      |
| 04 | 3155:1805        | 97.50          | 97.78          | 99.52         | 99.48          | 99.74    |
| 05 | 2420:2540        | 99.78          | 99.72          | 95.40         | 95.97          | 99.96    |
| 06 | 1879:3081        | 100            | 99.98          | 99.05         | 98.47          | 100      |
| 07 | 2673:2287        | 99.96          | 99.92          | 98.47         | 98.08          | 99.90    |
| 08 | 3803:1157        | 99.92          | 99.90          | 99.50         | 98.65          | 99.98    |
| 09 | 1558:3402        | 99.84          | 100            | 99.72         | 99.09          | 99.94    |
| 10 | 2319:2641        | 99.78          | 99.74          | 99.62         | 99.27          | 99.86    |
| 11 | 1709:3251        | 99.94          | 100            | 99.27         | 99.09          | 100      |
| 12 | 2676:2284        | 100            | 100            | 95.36         | 95.58          | 100      |
| 13 | 1740:3220        | 99.86          | 99.40          | 97.10         | 95.75          | 99.98    |
| 14 | 3156:1804        | 100            | 100            | 97.07         | 94.48          | 99.98    |
| 15 | 1132:3828        | 100            | 99.78          | 98.35         | 98.61          | 99.92    |
| 16 | 2153:2807        | 99.90          | 99.96          | 97.78         | 98.23          | 99.82    |
| 17 | 3079:1881        | 100            | 99.92          | 98.17         | 95.81          | 99.92    |
| 18 | 1916:3044        | 99.98          | 100            | 97.4          | 93.15          | 99.98    |
| 19 | 1200:3760        | 99.92          | 100            | 99.09         | 96.51          | 100      |
| 20 | 2107:2853        | 99.96          | 99.90          | 98.61         | 98.85          | 100      |
| 21 | 1367:3593        | 99.96          | 99.98          | 98.65         | 99.27          | 100      |
| 22 | 3079:1881        | 99.94          | 99.92          | 95.02         | 96.75          | 99.98    |
| 23 | 2887:2073        | 99.98          | 99.92          | 98.73         | 98.37          | 100      |

TABLE A.IV  
EXPERIMENTS WITH TEEGENDA WITH RHYTHM BAND COMPARISONS PERFORMED ON DEAP (0.5s-WINDOW, 0% OVERLAP).

| ID | No. Valence (0.5s) | LV/HV | No. of Arousal (0.5s) | LA/HA |
|----|--------------------|-------|-----------------------|-------|
| 01 | 2646:2394          | 100   | 2016:3024             | 100   |
| 02 | 2268:2772          | 96.31 | 2016:3024             | 96.49 |
| 03 | 2268:2772          | 95.10 | 4032:1008             | 93.77 |
| 04 | 3024:2016          | 89.64 | 3024:2016             | 89.19 |
| 05 | 2016:3024          | 98.41 | 2646:2394             | 97.54 |
| 06 | 1260:3780          | 99.90 | 2898:2142             | 100   |
| 07 | 1512:3528          | 100   | 1890:3150             | 100   |
| 08 | 2268:2772          | 99.29 | 2142:2898             | 99.38 |
| 09 | 2520:2520          | 98.91 | 2016:3024             | 98.49 |
| 10 | 2520:2520          | 98.69 | 2268:2772             | 99.56 |
| 11 | 2016:3024          | 91.63 | 3150:1890             | 91.19 |
| 12 | 2394:2646          | 99.90 | 882:4158              | 99.92 |
| 13 | 2898:2142          | 99.46 | 756:4284              | 99.25 |
| 14 | 2520:2520          | 99.72 | 1638:3402             | 98.27 |
| 15 | 2520:2520          | 99.56 | 2646:2394             | 99.70 |
| 16 | 3150:1890          | 99.90 | 2520:2520             | 99.98 |
| 17 | 2268:2772          | 99.96 | 2016:3024             | 99.62 |
| 18 | 2016:3024          | 99.90 | 1890:3150             | 99.84 |
| 19 | 2142:2898          | 99.54 | 1638:3402             | 99.07 |
| 20 | 2142:2898          | 99.76 | 1134:3906             | 99.68 |
| 21 | 2394:2646          | 98.59 | 1008:4032             | 97.22 |
| 22 | 2772:2268          | 92.04 | 2016:3024             | 92.08 |
| 23 | 1746:3276          | 100   | 3780:1260             | 99.80 |
| 24 | 2772:2268          | 99.13 | 882:4158              | 96.85 |
| 25 | 2646:2394          | 95.20 | 1386:3654             | 92.20 |
| 26 | 1764:3276          | 99.50 | 2898:2142             | 99.40 |
| 27 | 1260:3780          | 99.74 | 1638:3402             | 99.60 |
| 28 | 1890:3150          | 99.72 | 2772:2268             | 99.72 |
| 29 | 2142:2898          | 99.90 | 1890:3150             | 99.90 |
| 30 | 1638:3402          | 97.08 | 2646:2394             | 98.08 |
| 31 | 2142:2898          | 99.98 | 2646:2394             | 99.94 |
| 32 | 2520:2520          | 98.65 | 1638:3402             | 97.90 |

TABLE A.V  
EXPERIMENTS WITH TEEGND A WITH RHYTHM BAND COMPARISONS PERFORMED ON DEAP (2S-WINDOW, 25% OVERLAP).

| ID | No. Valence (2s) | LV/HV | No. of Arousal (2s) | LA/HA |
|----|------------------|-------|---------------------|-------|
| 01 | 903:817          | 99.83 | 688:1032            | 99.83 |
| 02 | 774:946          | 90.52 | 688:1032            | 92.21 |
| 03 | 774:946          | 89.36 | 334:1376            | 89.83 |
| 04 | 1032:688         | 87.67 | 1032:688            | 87.30 |
| 05 | 688:1032         | 95.47 | 903:817             | 96.05 |
| 06 | 430:1290         | 98.26 | 989:731             | 99.88 |
| 07 | 516:1204         | 99.71 | 645:1075            | 99.59 |
| 08 | 774:946          | 96.05 | 731:989             | 95.76 |
| 09 | 860:860          | 97.15 | 688:1032            | 97.50 |
| 10 | 860:860          | 96.40 | 774:946             | 96.86 |
| 11 | 688:1032         | 92.03 | 1075:645            | 88.49 |
| 12 | 817:903          | 98.84 | 301:1419            | 97.09 |
| 13 | 989:731          | 95.64 | 258:1462            | 98.43 |
| 14 | 860:860          | 96.34 | 559:1161            | 94.94 |
| 15 | 860:860          | 97.44 | 903:817             | 98.43 |
| 16 | 645:1075         | 98.95 | 860:860             | 99.42 |
| 17 | 774:946          | 98.72 | 688:1032            | 97.91 |
| 18 | 688:1032         | 99.01 | 645:1075            | 98.43 |
| 19 | 731:989          | 98.78 | 559:1161            | 97.62 |
| 20 | 731:989          | 98.60 | 387:1333            | 98.20 |
| 21 | 817:903          | 92.56 | 344:1376            | 92.85 |
| 22 | 946:774          | 88.66 | 688:1032            | 88.49 |
| 23 | 602:1118         | 99.59 | 1290:430            | 99.19 |
| 24 | 946:774          | 95.35 | 301:1419            | 92.79 |
| 25 | 903:817          | 91.63 | 473:1247            | 86.16 |
| 26 | 602:1118         | 98.02 | 989:731             | 99.19 |
| 27 | 430:1290         | 99.07 | 559:1161            | 98.78 |
| 28 | 645:1075         | 98.08 | 946:774             | 97.56 |
| 29 | 731:989          | 99.71 | 645:1075            | 99.53 |
| 30 | 559:1161         | 95.58 | 903:817             | 96.34 |
| 31 | 731:989          | 99.01 | 903:817             | 99.53 |
| 32 | 860:860          | 96.10 | 559:1161            | 94.65 |

TABLE A.VI  
EXPERIMENTS WITH TEEGENDA WITH RHYTHM BAND COMPARISONS PERFORMED ON DEAP (3S-WINDOW, 0% OVERLAP).

| ID | No. Valence (3s) | LV/HV | No. of Arousal (3s) | LA/HA |
|----|------------------|-------|---------------------|-------|
| 01 | 441:399          | 94.76 | 336:504             | 94.88 |
| 02 | 378:462          | 84.88 | 336:504             | 83.81 |
| 03 | 378:462          | 90.48 | 672:168             | 87.38 |
| 04 | 504:336          | 80.48 | 504:336             | 80.95 |
| 05 | 336:504          | 89.88 | 441:399             | 87.50 |
| 06 | 210:630          | 88.10 | 483:357             | 92.26 |
| 07 | 252:588          | 88.81 | 315:525             | 90.71 |
| 08 | 378:462          | 90.36 | 357:483             | 88.69 |
| 09 | 420:420          | 90.24 | 336:504             | 88.81 |
| 10 | 420:420          | 87.74 | 378:462             | 88.45 |
| 11 | 336:504          | 78.33 | 525:315             | 78.33 |
| 12 | 399:441          | 88.33 | 147:693             | 86.90 |
| 13 | 483:357          | 85.95 | 126:714             | 93.57 |
| 14 | 420:420          | 88.33 | 273:567             | 87.86 |
| 15 | 420:420          | 93.57 | 441:399             | 92.38 |
| 16 | 525:315          | 90.36 | 420:420             | 93.45 |
| 17 | 378:462          | 94.52 | 336:504             | 95.12 |
| 18 | 336:504          | 95.00 | 315:525             | 90.71 |
| 19 | 357:483          | 87.02 | 273:567             | 88.21 |
| 20 | 357:483          | 93.21 | 189:651             | 91.07 |
| 21 | 399:441          | 85.48 | 168:672             | 86.55 |
| 22 | 462:378          | 85.36 | 336:504             | 85.00 |
| 23 | 294:546          | 95.36 | 630:210             | 93.10 |
| 24 | 462:378          | 85.83 | 147:693             | 85.48 |
| 25 | 441:399          | 85.36 | 231:609             | 81.90 |
| 26 | 294:546          | 93.21 | 483:357             | 93.69 |
| 27 | 210:630          | 96.55 | 273:567             | 95.48 |
| 28 | 315:525          | 84.52 | 462:378             | 83.57 |
| 29 | 357:483          | 94.88 | 315:525             | 97.02 |
| 30 | 273:567          | 86.90 | 441:399             | 90.48 |
| 31 | 357:483          | 92.26 | 441:399             | 94.76 |
| 32 | 420:420          | 83.10 | 273:567             | 80.83 |

TABLE A.VII  
EXPERIMENTS WITH TEEGND A WITH RHYTHM BAND COMPARISONS PERFORMED ON DEAP (4S-WINDOW, 25% OVERLAP).

| ID | No. Valence (4s) | LV/HV | No. of Arousal (4s) | LA/HA |
|----|------------------|-------|---------------------|-------|
| 01 | 441:399          | 95.71 | 336:504             | 95.48 |
| 02 | 360:440          | 83.13 | 320:480             | 83.37 |
| 03 | 360:440          | 88.00 | 640:160             | 86.88 |
| 04 | 480:320          | 83.25 | 480:320             | 82.25 |
| 05 | 320:480          | 88.38 | 420:380             | 86.88 |
| 06 | 200:600          | 85.75 | 460:340             | 86.62 |
| 07 | 240:560          | 83.25 | 300:500             | 87.75 |
| 08 | 360:440          | 91.13 | 340:460             | 89.75 |
| 09 | 400:400          | 93.50 | 320:480             | 87.00 |
| 10 | 400:400          | 89.88 | 360:440             | 87.75 |
| 11 | 320:480          | 84.12 | 500:300             | 77.37 |
| 12 | 380:420          | 88.25 | 140:660             | 88.25 |
| 13 | 460:340          | 87.13 | 120:680             | 92.25 |
| 14 | 400:400          | 87.25 | 260:540             | 86.62 |
| 15 | 400:400          | 94.25 | 420:380             | 93.88 |
| 16 | 500:300          | 90.88 | 400:400             | 93.00 |
| 17 | 360:440          | 93.63 | 320:480             | 94.37 |
| 18 | 320:480          | 84.25 | 300:500             | 89.50 |
| 19 | 340:460          | 87.75 | 260:540             | 86.38 |
| 20 | 340:460          | 92.55 | 180:620             | 89.87 |
| 21 | 380:420          | 85.25 | 160:640             | 86.12 |
| 22 | 440:360          | 83.75 | 320:480             | 86.12 |
| 23 | 280:520          | 95.75 | 600:200             | 93.13 |
| 24 | 440:360          | 83.00 | 140:660             | 85.50 |
| 25 | 420:380          | 84.25 | 220:580             | 80.75 |
| 26 | 280:520          | 93.62 | 460:340             | 93.00 |
| 27 | 200:600          | 95.00 | 260:540             | 95.63 |
| 28 | 300:500          | 83.00 | 440:360             | 84.50 |
| 29 | 340:460          | 95.25 | 300:500             | 94.12 |
| 30 | 260:540          | 86.37 | 420:380             | 88.75 |
| 31 | 340:460          | 93.62 | 420:380             | 90.62 |
| 32 | 400:400          | 85.50 | 260:540             | 80.88 |

TABLE A.VIII  
EXPERIMENTS WITH TEEGND A WITH WINDOW LENGTH COMPARISONS PERFORMED ON DREAMER WITH ALL-FOUR-BANDS (0.5S-WINDOW, 0%OVERLAP)

| ID | No. Valence-0.5s | LV/HV(%) | No. Arousal-0.5s | LA/HA(%) | No. Dominance-0.5s | LD/HD(%) |
|----|------------------|----------|------------------|----------|--------------------|----------|
| 01 | 3950:3506        | 99.83    | 5116:2340        | 99.91    | 2940:4516          | 99.91    |
| 02 | 5086:2370        | 99.84    | 3130:4326        | 99.99    | 2880:4576          | 99.93    |
| 03 | 3818:3638        | 99.97    | 3972:3484        | 100      | 4392:3064          | 97.42    |
| 04 | 5724:1732        | 99.60    | 5126:2330        | 99.69    | 4744:2712          | 99.70    |
| 05 | 4688:2768        | 99.85    | 3368:4088        | 99.77    | 3640:3816          | 99.85    |
| 06 | 4052:3404        | 99.99    | 2292:5164        | 99.96    | 2826:4630          | 99.95    |
| 07 | 4888:2568        | 99.96    | 4498:2958        | 100      | 4020:3436          | 99.99    |
| 08 | 4928:2528        | 100      | 5374:2082        | 99.93    | 5718:1738          | 100      |
| 09 | 4162:3294        | 99.97    | 2080:5376        | 100      | 2342:5114          | 99.97    |
| 10 | 2808:4648        | 99.91    | 4590:2866        | 99.84    | 3486:3970          | 99.75    |
| 11 | 4814:2642        | 99.96    | 4236:3220        | 99.99    | 2570:4886          | 100      |
| 12 | 3646:3810        | 99.99    | 3796:3660        | 99.96    | 4024:3432          | 99.99    |
| 13 | 3252:4204        | 99.96    | 3746:3710        | 99.99    | 2618:4838          | 99.97    |
| 14 | 4144:3312        | 99.97    | 4564:2892        | 100      | 4744:2712          | 99.97    |
| 15 | 4888:2568        | 99.68    | 3476:3980        | 99.88    | 1702:5754          | 99.91    |
| 16 | 4696:2760        | 99.81    | 3378:4078        | 99.75    | 3238:4218          | 99.81    |
| 17 | 4824:2632        | 99.95    | 5294:2162        | 99.97    | 4630:2826          | 99.97    |
| 18 | 4696:2760        | 99.95    | 3232:4224        | 100      | 2882:4574          | 99.99    |
| 19 | 3546:3910        | 99.92    | 1202:6254        | 99.91    | 1804:5652          | 99.92    |
| 20 | 4994:2462        | 99.99    | 4628:2828        | 99.97    | 3168:4288          | 99.96    |
| 21 | 4670:2786        | 99.99    | 2328:5128        | 100      | 2056:5400          | 99.99    |
| 22 | 4710:2746        | 99.96    | 4706:2750        | 99.96    | 4628:2828          | 100      |
| 23 | 4036:3420        | 100      | 5178:2278        | 100      | 4342:3114          | 100      |

TABLE A.IX  
EXPERIMENTS WITH TEEGND A WITH WINDOW LENGTH COMPARISONS PERFORMED ON DREAMER WITH ALL-FOUR-BANDS (2S-WINDOW, 25% OVERLAP)

| ID | No. Valence-2s | LV/HV(%) | No. Arousal-2s | LA/HA(%) | No. Dominance-2s | LD/HD(%) |
|----|----------------|----------|----------------|----------|------------------|----------|
| 01 | 1381:1225      | 99.66    | 1787:819       | 99.58    | 1027:1579        | 99.77    |
| 02 | 1777:829       | 99.81    | 1093:1513      | 99.88    | 1005:1601        | 99.58    |
| 03 | 1334:1272      | 100      | 1387:1219      | 99.88    | 1533:1073        | 100      |
| 04 | 2000:606       | 99.35    | 1791:815       | 99.58    | 1657:949         | 99.42    |
| 05 | 1638:968       | 99.77    | 1176:1430      | 99.77    | 1270:1336        | 99.77    |
| 06 | 1416:1190      | 99.92    | 801:1805       | 99.96    | 987:1619         | 99.88    |
| 07 | 1708:898       | 99.23    | 1572:1034      | 99.85    | 1405:1201        | 99.73    |
| 08 | 1722:884       | 99.73    | 1878:728       | 99.69    | 1998:608         | 99.92    |
| 09 | 1455:1151      | 99.96    | 727:1879       | 99.92    | 818:1788         | 99.85    |
| 10 | 982:1624       | 99.65    | 1604:1002      | 99.58    | 1217:1389        | 99.39    |
| 11 | 1682:924       | 99.92    | 1480:1126      | 100      | 898:1708         | 100      |
| 12 | 1274:1332      | 99.62    | 1326:1280      | 99.73    | 1406:1200        | 99.88    |
| 13 | 1137:1469      | 99.77    | 1308:1298      | 99.58    | 913:1693         | 99.39    |
| 14 | 1448:1158      | 99.88    | 1594:1012      | 99.96    | 1657:949         | 99.89    |
| 15 | 1708:898       | 99.19    | 1214:1392      | 99.81    | 595:2011         | 99.39    |
| 16 | 1641:965       | 99.65    | 1179:1427      | 99.62    | 1130:1476        | 99.58    |
| 17 | 1686:920       | 99.42    | 1850:706       | 99.92    | 1619:987         | 99.89    |
| 18 | 1641:965       | 99.73    | 1128:1478      | 99.88    | 1006:1600        | 99.62    |
| 19 | 1239:1367      | 99.50    | 419:2187       | 99.46    | 629:1977         | 99.77    |
| 20 | 1746:860       | 99.96    | 1617:989       | 100      | 1107:1499        | 99.81    |
| 21 | 1631:975       | 99.96    | 812:1794       | 99.96    | 718:1888         | 100      |
| 22 | 1647:959       | 99.81    | 1644:962       | 99.88    | 1618:988         | 99.77    |
| 23 | 1410:1196      | 99.81    | 1810:796       | 99.96    | 1517:1089        | 99.96    |

TABLE A.X

EXPERIMENTS WITH TEEGND A WITH WINDOW LENGTH COMPARISONS PERFORMED ON DREAMER WITH ALL-FOUR-BANDS (3s-WINDOW, 0% OVERLAP)

| ID | No. Valence-3s | LV/HV(%) | No. Arousal-3s | LA/HA(%) | No. Dominance-3s | LD/HD(%) |
|----|----------------|----------|----------------|----------|------------------|----------|
| 01 | 655:582        | 99.35    | 848:389        | 98.87    | 487:750          | 99.43    |
| 02 | 843:394        | 99.60    | 519:718        | 99.68    | 477:760          | 99.35    |
| 03 | 633:604        | 99.43    | 659:578        | 99.19    | 728:509          | 99.92    |
| 04 | 949:288        | 98.95    | 850:387        | 99.27    | 786:451          | 99.35    |
| 05 | 777:460        | 99.43    | 558:679        | 98.71    | 603:634          | 99.11    |
| 06 | 671:566        | 99.60    | 380:857        | 99.76    | 468:769          | 99.68    |
| 07 | 810:427        | 98.79    | 746:491        | 99.51    | 667:570          | 99.03    |
| 08 | 817:420        | 99.03    | 892:345        | 99.43    | 949:288          | 99.68    |
| 09 | 690:547        | 99.60    | 345:892        | 99.60    | 388:849          | 99.51    |
| 10 | 465:772        | 99.19    | 761:476        | 99.03    | 577:660          | 99.27    |
| 11 | 798:439        | 99.76    | 703:534        | 99.84    | 426:811          | 99.92    |
| 12 | 604:633        | 99.27    | 630:607        | 97.90    | 667:570          | 99.84    |
| 13 | 539:698        | 98.71    | 621:616        | 99.03    | 434:803          | 98.87    |
| 14 | 687:550        | 100      | 756:481        | 99.92    | 786:451          | 99.84    |
| 15 | 810:427        | 98.95    | 576:661        | 98.63    | 282:955          | 98.87    |
| 16 | 778:450        | 99.35    | 559:678        | 99.19    | 536:701          | 99.03    |
| 17 | 800:437        | 99.11    | 878:359        | 99.43    | 768:469          | 98.87    |
| 18 | 778:459        | 98.95    | 536:701        | 99.43    | 478:759          | 99.99    |
| 19 | 588:649        | 98.62    | 199:1038       | 98.95    | 298:939          | 99.11    |
| 20 | 828:409        | 98.54    | 767:470        | 99.60    | 525:712          | 99.60    |
| 21 | 774:463        | 99.76    | 386:851        | 99.03    | 341:896          | 99.27    |
| 22 | 781:456        | 99.43    | 780:457        | 99.51    | 767:470          | 99.68    |
| 23 | 669:568        | 99.19    | 859:378        | 99.76    | 720:517          | 99.68    |

TABLE A.XI

EXPERIMENTS WITH TEEGND A WITH WINDOW LENGTH COMPARISONS PERFORMED ON DREAMER WITH ALL-FOUR-BANDS (4s-WINDOW, 25% OVERLAP)

| ID | No. Valence-4s | LV/HV(%) | No. Arousal-4s | LA/HA(%) | No. Dominance-4s | LD/HD(%) |
|----|----------------|----------|----------------|----------|------------------|----------|
| 01 | 653:579        | 99.35    | 846:386        | 98.78    | 485:747          | 99.51    |
| 02 | 841:391        | 99.59    | 517:715        | 99.59    | 475:757          | 99.27    |
| 03 | 632:600        | 99.67    | 655:577        | 99.68    | 724:508          | 99.76    |
| 04 | 946:286        | 98.62    | 846:386        | 99.11    | 783:449          | 99.35    |
| 05 | 775:457        | 99.35    | 556:676        | 99.59    | 600:632          | 99.51    |
| 06 | 671:561        | 99.59    | 378:854        | 99.43    | 466:766          | 99.51    |
| 07 | 808:427        | 98.46    | 742:490        | 99.43    | 663:569          | 99.19    |
| 08 | 815:417        | 99.03    | 888:344        | 98.95    | 944:288          | 99.59    |
| 09 | 689:543        | 99.51    | 344:888        | 99.76    | 387:845          | 99.51    |
| 10 | 465:767        | 99.35    | 759:473        | 99.19    | 576:656          | 99.03    |
| 11 | 796:436        | 99.51    | 699:533        | 99.92    | 424:808          | 99.92    |
| 12 | 603:629        | 98.94    | 626:606        | 98.05    | 664:568          | 99.59    |
| 13 | 538:694        | 98.78    | 618:614        | 99.19    | 431:801          | 98.30    |
| 14 | 686:546        | 99.59    | 754:478        | 99.67    | 784:448          | 99.76    |
| 15 | 808:424        | 98.70    | 574:658        | 98.46    | 281:951          | 98.95    |
| 16 | 777:455        | 99.19    | 558:674        | 99.19    | 534:698          | 99.43    |
| 17 | 798:434        | 98.54    | 874:358        | 99.19    | 764:468          | 98.70    |
| 18 | 777:455        | 99.19    | 533:699        | 99.43    | 475:757          | 99.35    |
| 19 | 587:645        | 98.87    | 199:1033       | 98.78    | 298:934          | 99.11    |
| 20 | 826:406        | 97.81    | 765:467        | 99.92    | 523:709          | 99.19    |
| 21 | 772:460        | 99.59    | 383:849        | 98.86    | 339:893          | 99.35    |
| 22 | 779:453        | 99.03    | 777:455        | 99.51    | 765:467          | 99.68    |
| 23 | 667:565        | 99.03    | 855:377        | 99.76    | 716:516          | 99.76    |
